# Supplementary material for: Improving the Robustness of Quantized Deep Neural Networks to White-Box Attacks using Stochastic Quantization and Information-Theoretic Ensemble Training
Source: arXiv:2312.00105 source file (2023-11-30)
Supplement: Supplementary file 1 [file 8_appendix.tex]

\section*{Appendix}

\textbf{\small Data:}
$X=\{X_1,X_2\}\in[0,1]\times[0,1]$

\textbf{\small Sample:}
$x=\{x_1=0.7,x_2=0.6\}$

\textbf{\small DNN Assumed:}
$x\rightarrow X\rightarrow \tilde{x}\rightarrow \hat{W} \rightarrow t\rightarrow T\rightarrow \tilde{t}\rightarrow y$

\[
W=\begin{pmatrix}
0.5 & 0.4 \\
0.3 & 0.2
\end{pmatrix}
\]

So, 
\[
t=\begin{pmatrix}
t_1 \\
t_2
\end{pmatrix}=
\begin{pmatrix}
0.5x_1+0.3x_2 \\
0.4x_1+0.2x_2
\end{pmatrix}
\]

\textbf{\small Quantized Input Distribution:}

\begin{center}
\fbox{%
\begin{tabular}{c|c|c}
$X_i$ & $P(X_i=0)$ & $P(X_i=1)$ \\
\hline
$X_1$ & 0.3 & 0.7 \\
$X_2$ & 0.4 & 0.6 \\
\end{tabular}%
}
\end{center}

\textbf{\small Quantized Feature Distribution:}

\begin{center}
\fbox{%
\begin{tabular}{c|c|c}
$T_i$ & $P(T_i=0)$ & $P(T_i=1)$ \\
\hline
$T_1$ & $1-t_1$ & $t_1$ \\
$T_2$ & $1-t_2$ & $t_2$ \\
\end{tabular}%
}
\end{center}

\textbf{\small Conditional Distribution for $T_1$:}

\begin{center}
\fbox{%
\begin{tabular}{c|cccc}
$T_1 |x_1,x_2$ & 00 & 01 & 10 & 11 \\
\hline
$T_1=0$ & 1 & 0.7 & 0.5 & 0.2 \\
$T_1=1$ & 0 & 0.3 & 0.5 & 0.8 \\
\end{tabular}%
}
\end{center}

\textbf{\small Conditional Distribution for $T_2$:}

\begin{center}
\fbox{%
\begin{tabular}{c|cccc}
$T_2 |x_1,x_2$ & 00 & 01 & 10 & 11 \\
\hline
$T_2=0$ & 1 & 0.8 & 0.6 & 0.4 \\
$T_2=1$ & 0 & 0.2 & 0.4 & 0.6 \\
\end{tabular}%
}
\end{center}

\textbf{Marginal distribution for $T_1$: $p(T)=\sum_{x\in\text{samples}} p(x)p(T|x)$}

\begin{center}
\fbox{%
\begin{tabular}{@{}cccccc@{}}
            & $X_1,X_2=0,0$ & $X_1,X_2=0,1$ & $X_1,X_2=1,0$ & $X_1,X_2=1,1$ & $P(T_1)$ \\
            \hline
            $P(T_1=0)$ & $0.3\times0.4$ & $0.7\times0.3\times0.6$ & $0.5\times0.7\times0.4$ & $0.2\times0.7\times0.6$ & $0.47$ \\
            $P(T_2=0)$ & $0$ & $0.3\times0.3\times0.6$ & $0.5\times0.7\times0.4$ & $0.8\times0.7\times0.6$ & $0.53$ \\
\end{tabular}%
}
\end{center}
